# Supplementary material for: A Multiversion Programming Inspired Approach to Detecting Audio Adversarial Examples
Source: arXiv:1812.10199 source file (2019-12-03)
Supplement: Supplementary file 1 [file appendix.tex]

\begin{table*}[!ht]
    \centering
    \caption{Experiment results of the concatenating attack. In order to generate transferable audio AE that can attack two ASR systems. We first tamper a host audio sample with the stage 1 attack targeting the ASR system 1. Then the outputted intermediate AE sample is further manipulated by the stage 2 attack targeting the ASR system 2. We embed the same text for two both two stages. The final generated AE samples are evaluated about their transferability by transcripted by two targeting ASR systems respectively and calculate the phonetic similarity score (PSS) between two transcriptions. We have three attacking tools in total: CS represents the CommanderSong~\cite{DBLP:conf/uss/YuanCZLL0ZH0G18}, WB and BB are Whitebox~\cite{DBLP:conf/sp/Carlini018} and Blackbox~\cite{DBLP:journals/corr/abs-1805-07820} attack respectively.For the target ASR systems, we have  Kaldi denoted as kd and deepspeech version 0.1.0 and 0.1.1 denoted as ds0 and ds1 respectively.}

    \begin{tabu} to \hsize {|X[0.7]|X[3]|X|X|X[3]|X[3]|X[3]|X[0.5]|}
    \hline
    \multicolumn{2}{|c|}{Host Audio Sample}&\multicolumn{3}{c|}{Attacks}&\multicolumn{3}{c|}{Evaluation} \\ \hline
    Name&Host Transcription &Stage1&Stage2&Target Text&ASR1 Transcription&ASR2 Transcription&PSS \\ 
    % \tabucline[1.5pt]{-}
    \hhline{|=|=|=|=|=|=|=|=|}

    CS1&song&CS-kd& WB-ds0&okay google turn on g. p. s. the guy& okay google turn on g. p. s. the guy in yeah & okay google turn on gps &0.92 \\ \hline
    
    CS2&song&CS-kd& WB-ds0&okay google call one one zero one one nine one two zero& okay google call one one zero one one nine one two zero & okay google call one one zero one one nine one to zero &0.85 \\ \hline
    
    CSW1&song&CS-kd& WB-ds0&echo open the front door& open door uh & to open the front door &0.61 \\ \hline
    
    CSW2 &song&CS-kd& WB-ds0&okay google clear notification wild inter cell in marin it's & okay google clearly nato god i don't think there's no in marin it's & okay google clear notification wild inter cell in marin it &0.87 \\ \hline
    
    CSW3 &song&CS-kd& WB-ds0&okay google call one one zero one one nine one two zero manner & okay google one one two zero manner & okay google call one one to one one in one to zero manner &0.83 \\ \hline
    
    CSW4 &song&CS-kd& WB-ds0&okay google turn on g. p. s. h. a. diane reid & uh okay angie and i'm in uh oh god in [noise] read & okay google turn on gps a diane reid &0.68 \\ \hline
    
    CSW5 &song&CS-kd& WB-ds0&okay google good night will oh we're neighbors around i spend & okay good will the way we're an hour at age says it & okay good good night will oh we are neighbors around i spend &0.68 \\ \hline
    
    WW1 &without the dataset the article is useless&WB-ds0& WB-ds1&enough said the boy & witovetheesaid therybusesis & enough said the boy &0.51 \\ \hline
    
    WW2 &without the dataset the article is useless&WB-ds0& WB-ds1&a sight for sore eyes & atabedtetisitbeordhoreeistis & a sight for sore eyes &0.55 \\ \hline
    
    WW3 &without the dataset the article is useless&WB-ds0& WB-ds1&everyone seemed very excited & tevertatesedheare blysuswlitsad & every one seemed very excited &0.58 \\ \hline
    
    WW4 &without the dataset the article is useless&WB-ds0& WB-ds1&plastic surgery has become more popular & lithautthergav ishadbeanporseoleri & plastic surgery has become more popular &0.60 \\ \hline
    
    WW5 &without the dataset the article is useless&WB-ds0& WB-ds1&i can learn something from the desert too & i outlertattherfro mtheardqueseuspoos & i can learn something from the desert too &0.76 \\ \hline
    
    BB1 &without the dataset the article is useless&BB-ds0& BB-ds1&side laugh & orvavadesairdleargrcesith & side laugh &0.53 \\ \hline
    
    BB2 &without the dataset the article is useless&BB-ds0& BB-ds1&president together & apresiegottotoho & president together &0.69 \\ \hline
    
    BB3 &without the dataset the article is useless&BB-ds0& BB-ds1&draw sure & and now & draw sure &0.57 \\ \hline
    
    BB4 &without the dataset the article is useless&BB-ds0& BB-ds1&it think & so thou & it think &0.66 \\ \hline
    
    BB5 &without the dataset the article is useless&BB-ds0& BB-ds1&firm late & holdyornos dicithismell fomthisal agerotobarcol & firm late &0.44 \\ \hline

    WB1 &without the dataset the article is useless&WB-ds0& BB-ds1&enough said the boy & rtotehasaid hearegoseusirs & enough said the boy &0.29 \\ \hline
    
    WB2 &without the dataset the article is useless&WB-ds0& BB-ds1&a sight for sore eyes & erhatte vatihe & a sight for sore eyes &0.38 \\ \hline
    
    WB3 &without the dataset the article is useless&WB-ds0& BB-ds1&everyone seemed very excited & orveverthataser veardvorithysfit & every one seemed very excited &0.55 \\ \hline
    
    WB4 &without the dataset the article is useless&WB-ds0& BB-ds1&plastic surgery has become more popular & i was out the batishavet heardworstestir & plastic surgery has become more popular &0.53 \\ \hline
    
    WB5 &without the dataset the article is useless&WB-ds0& BB-ds1&i can learn something from the desert too & what other that of to the ariquece yousedto & i can learn something from the desert too &0.67 \\ \hline

    BW1 &most meteorites are more&BB-ds0& WB-ds1&material every & monever ieowyerletma & material every &0.56 \\ \hline
    
    BW2 &it's candice now on long distance from washington &BB-ds0& WB-ds1&price something & apresiegottotoho & pricesoething &0.71 \\ \hline
    
    BW3 &he could always go back to being a shepherd &BB-ds0& WB-ds1&board let & and now & board let &0.6 \\ \hline
    
    BW4 &it seemed so safe and tranquil&BB-ds0& WB-ds1&beyond ok & wiesilsaendwank & ben &0.53 \\ \hline
    
    BW5 &their faces were hidden behind blue veils with only their eyes showing &BB-ds0& WB-ds1&husband little & that a is lefidinbehind lothereleiye & husband little &0.56 \\ \hline

    \end{tabu}
    \label{table:concatenation}
\end{table*}
